# Supplementary material for: Spin-Orbit Protection of Induced Superconductivity in Majorana Nanowires
Source: arXiv:1807.01940 ancillary file (2019-05-10)
Supplement: Supplementary file 1 [file Supplemental_Material.pdf]

# Supplemental Material: Spin-Orbit Protection of Induced Superconductivity in Majorana Nanowires

Jouri D.S. Bommer,[1,2] Hao Zhang,[1,2,3,*] Önder Gül,[1,2,†] Bas Nijholt,[2] Michael Wimmer,[1,2] Filipp N. Rybakov,[4] Julien Garaud,[5] Donjan Rodic,[6] Egor Babaev,[4] Matthias Troyer,[6,7] Diana Car,[8] Sébastien R. Plissard,[8,‡] Erik P.A.M. Bakkers,[1,2,8] Kenji Watanabe,[9] Takashi Taniguchi,[9] and Leo P. Kouwenhoven[1,2,10]

[1] *QuTech, Delft University of Technology, 2600 GA Delft, The Netherlands*
[2] *Kavli Institute of Nanoscience, Delft University of Technology, 2600 GA Delft, The Netherlands*
[3] *State Key Laboratory of Low Dimensional Quantum Physics, Department of Physics, Tsinghua University, Beijing 100084, China*
[4] *Department of Physics, KTH-Royal Institute of Technology, SE-10691 Stockholm, Sweden*
[5] *Laboratoire de Mathématiques et Physique Théorique CNRS/UMR 7350, Institut Denis Poisson FR2964, Université de Tours, Parc de Grandmont, 37200 Tours, France*
[6] *Institut für Theoretische Physik, ETH Zürich, 8093 Zürich, Switzerland*
[7] *Microsoft Quantum, Redmond, WA 98052, USA*
[8] *Department of Applied Physics, Eindhoven University of Technology, 5600 MB Eindhoven, The Netherlands*
[9] *Advanced Materials Laboratory, National Institute for Materials Science, 1-1 Namiki, Tsukuba, 305-0044, Japan*
[10] *Microsoft Station Q Delft, 2600 GA Delft, The Netherlands*

## CONTENTS

Supplemental Experimental Details 2
Nanowire growth and device fabrication 2
Measurement details 2

Supplemental Theoretical Details 3
Details of the tight binding simulations 3
Details of the Ginzburg-Landau simulations 3

Extraction of SOI strength 5
Determination of SOI strength $\alpha$ from gap closing 5
Estimation of SOI strength based on level repulsion 6

Supplemental Experimental Data 8

References 12

* HaoZhangDelft@gmail.com
† Present address: Department of Physics, Harvard University, Cambridge, MA 02138, USA
‡ Present address: CNRS-Laboratoire d'Analyse et d'Architecture des Systèmes (LAAS), Université de Toulouse, 7 avenue du colonel Roche, F-31400 Toulouse, France

## SUPPLEMENTAL EXPERIMENTAL DETAILS

### Nanowire growth and device fabrication

The InSb nanowires used here were grown using a Au-catalysed vapor-liquid-solid mechanism in a metal organic vapor phase epitaxy reactor, resulting in zinc blende nanowires grown along the [111] crystal orientation, which are free of stacking faults and dislocations [1]. Local gates, covered by a h-BN dielectric flake, were fabricated on a silicon substrate. The nanowires were individually placed over the gates using a micromanipulator [2]. The contacts are fabricated by exposing the chip to a mild oxygen plasma cleaning after resist development, followed by immersion in a saturated ammonium polysulphide solution diluted by water to a 1:200 ratio for 30 minutes at 60°C [3]. For the normal contacts, the wires are exposed to 30 seconds of in-situ helium ion milling, before evaporating 10 nm Cr and 110 nm Au. The NbTiN contacts are fabricated by exposing the nanowire to 5 seconds or Ar plasma etching at 25 W, followed by sputtering of 5 nm NbTi and 85 nm NbTiN [4, 5].

### Measurement details

The measurements were performed in a dilution refrigerator at an electron temperature of $\sim$ 50 mK using a three-axis vector magnet and standard lockin techniques.

# SUPPLEMENTAL THEORETICAL DETAILS

## Details of the tight binding simulations

The Hamiltonian defined in the main text is discretized on a lattice of a realistic nanowire geometry with a diameter of 70 nm and a length of 2 $\mu$m using a lattice spacing of 10 nm. The nanowire is covered by a 35 nm thick superconducting shell covering 3/8 of the circumference of the wire, posititioned on top of the wire [Fig. 2, 3(b)] or rotated from the top to the side by 45° [Fig. 4(b)]. Transport calculations are performed by connecting the nanowire to semi-infinite normal leads, separated by a tunnel barrier on one side. The normal leads provide broadening of the peaks in the simulations [6, 7]. The superconducting proximity effect is implemented using the weak coupling approximation [8], in which the pairing gap $\Delta_0 = 0$ in the nanowire, which is tunnel coupled to a superconductor with $\Delta_0 > 0$ providing an induced gap of 0.45 meV at $B = 0$ T. The potential in the wire is given by $V(y, z) = \frac{\Delta V_G}{R}(z\cos(\Phi) + y\sin(\Phi))$, where $\Delta V_G$ is the potential difference between the middle and outer points of the wire, $R$ is the radius of the nanowire, and $\Phi$ parametrizes the direction of the electric field $\hat{\mathbf{E}}$, which is set to $\Phi = 0°$ in all simulations, except for Fig. 4(d), where $\Phi = 45°$. The vector potential $\mathbf{A} = [B_y(z - z_0) - B_z(y - y_0), 0, B_x(y - y_0)]^T$ is chosen such that it does not depend on $x$ and the offsets $x_0$, $y_0$, $z_0$ are chosen such that the vector potential averages to zero inside the superconductor, implying a total supercurrent of zero in the superconductor. This choice is supported by the negligible screening currents we observe in our Ginzburg-Landau simulations [Fig. S1]. $\mathbf{A}$ is implemented in the tight-binding model by Peierls substitution in the hopping amplitudes [9].

## Details of the Ginzburg-Landau simulations

To calculate the stray fields in the nanowire due to Meissner screening and vortex entry in the superconducting contact (results shown in Fig. S1), we have performed simulations on the Ginzburg-Landau model [10] in a realistic three-dimensional geometry using the dimensions of device A. We used a penetration depth $\lambda = 290$ nm and a Ginzburg-Landau parameter $\kappa = \lambda/\xi = 50$, in line with the values expected for our NbTiN film, which has a room temperature resistivity of 95 $\mu\Omega$cm and a critical temperature of 15 K. The Ginzburg-Landau functional is discretized both inside the superconducting contact as well as in its surrounding space [11] using a second-order finite difference scheme at a maximum internode distance of $0.01\lambda$. The resulting energy functional is minimized using the nonlinear conjugate gradient method and the code is implemented on a NVidia CUDA architecture with high parallelization. We obtain the energy of states with vortices at finite magnetic fields by first introducing artificial perturbations near the sample boundary, followed by energy minimization to find the local minimum corresponding to a specific number of vortices. The optimal number of vortices at a certain magnetic field is then determined by finding the state with the lowest energy globally. We note that non-optimal amounts of vortices can be metastable due to significant Bean-Livingston barriers for vortex entry, so the actual number of vortices is hysteretic and depends on the dynamics of the magnetic field.

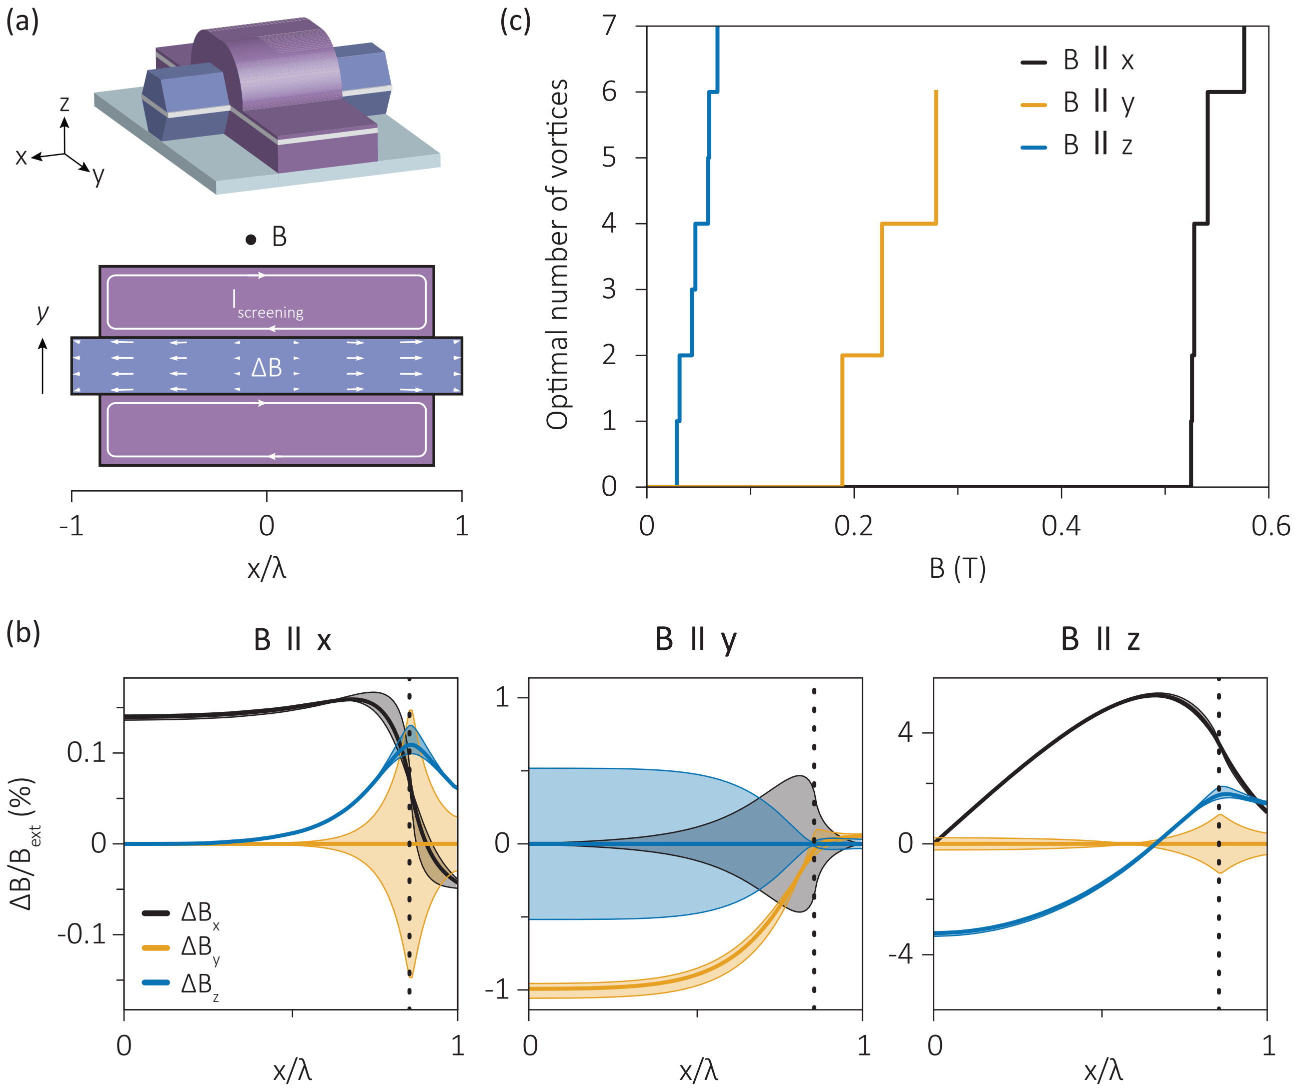


FIG. S1. Ginzburg-Landau simulations. (a) The top panel shows the schematic of the geometry used for Ginzburg-Landau simulations: a superconducting film covering a hexagonal nanowire. In a superconductor exposed to an external magnetic field $B$ we calculate the screening currents $I_{\mathrm{screening}}$, which induce stray magnetic fields $\Delta B$ in the nanowire. In (b) we show $\Delta B$ in the $xy$-plane in the middle of the nanowire, as indicated by the white line in (a). The bottom panel shows a top view of this $xy$-plane, where the arrows indicate the $x$ and $y$ components of $\Delta B$ in the nanowire for $B \parallel z$. (b) The $x$, $y$ and $z$-components (black, yellow, blue) of $\Delta B$ relative to the external field $B$ as a function of the position $x$ along the nanowire axis, where $x = 0$ corresponds to the middle of the superconducting contact. The lines show the mean stray field and the shaded regions are bounded by the minimum and maximum stray field found along the nanowire width at a particular $x$. The end of the superconducting film is indicated by the dashed line. $B$ is along $x$, $y$ and $z$ (left, middle and right panel). Since the device dimensions are comparable to the penetration depth $\lambda = 290$ nm, the magnetic screening in the superconductor is incomplete, leading to small screening currents and stray fields of at most 4% of $B$. These modifications are much smaller and do not match the anisotropy we observe in the measurements, which excludes Meissner screening as the origin of the observed anisotropic gap closing. We note that we have also evaluated $\Delta B$ at several different magnitudes of $B$ as well as in the presence of vortices and find relative stray fields of very comparable magnitude. (c) Energetically most favorable number of vortices as a function of $B$ along $x$, $y$ and $z$ (black, yellow, blue). Vortices form far more easily for $B \parallel z$. An anisotropic gap closing due to vortices near the nanowire would therefore cause the fastest gap closing along $z$, contrary to the anisotropic gap closing we observe, where the gap closes fastest for $B \parallel y$ [see e.g. Fig. 1(e)]. Furthermore, for $B \parallel y$ vortices only start to appear at $B > 0.2$ T, while the gap is already strongly suppressed at 0.2 T [see e.g. Fig. 1(e)], which excludes vortex formation as the origin of the gap closing for $B \parallel y$ and indicates that vortices do not have a strong effect on the size of the induced gap.

## EXTRACTION OF SOI STRENGTH

### Determination of SOI strength $\alpha$ from gap closing

In a Majorana nanowire the SOI strength $\alpha$ determines the shape of the gap closing along $B$-directions perpendicular to the spin-orbit field $B_{\mathrm{SO}}$ [12, 13] [see Fig. S2(a)]. To find an analytical expression for the dependence of the gap closing on $\alpha$, we start from the conventional one-dimensional Majorana nanowire Hamiltonian [14, 15], in which the gap size is given by the lowest energy eigenstate:

$$\Delta(B) = \min\left(\epsilon^2 + \epsilon_{\mathrm{SO}}^2 + \epsilon_Z^2 + \Delta(0)^2 \pm 2\sqrt{\epsilon^2(\epsilon_{\mathrm{SO}}^2 + \epsilon_Z^2) + \epsilon_Z^2\Delta(0)^2}\right)^{\frac{1}{2}} \tag{S1}$$

Here, $\epsilon = \hbar^2k^2/2m^* - \mu$ represents the kinetic energy, with $k$ the electron wave vector and $m^* = 0.015m_e$ the effective mass. $\epsilon_{\mathrm{SO}} = \alpha k$ is the SOI term with $\alpha$ the SOI strength. $\epsilon_Z = \frac{1}{2}g\mu_B B$ is the Zeeman energy, with $g$ the Landé $g$-factor and $\mu_B$ the Bohr magneton. $\Delta(0)$ is the induced superconducting gap at $B = 0$ T, which we measure in the experiments (as indicated in Fig. 1(b)).

For $B \parallel B_{\mathrm{SO}}$ ($y$-axis) and neglecting the orbital effect the gap closes linearly with the Zeeman energy due to tilting of the bands [16, 17]:

$$\Delta(B) = \Delta(0) - \frac{1}{2}g\mu_B B \tag{S2}$$

The orbital effect significantly enhances the gap closing in our devices [cf. Fig. 1,2], with a strong dependence on the potential difference $\Delta V_G$ in the three-dimensional model. Although the value of $\Delta V_G$ in our devices is unknown, we find that the orbital effect can be effectively taken into account in the one-dimensional model by adjusting the $g$-factor to match the gap closing along $B_{\mathrm{SO}}$, where SOI disappears and only the Zeeman and orbital effect contribute to the gap closing. We emphasize that the $g$-factor extracted from the fits therefore does not correspond to the pure Zeeman $g$-factor used in our tight-binding calculations. The validity of this approximation is demonstrated in Fig. S2(b), where the color map shows the gap closing resulting from our numerical calculations on the three-dimensional tight-binding model (taking the orbital effect into account and using $g = 50$) and the dashed white lines show the gap given by equation (S1) for $B \parallel x$ and by equation (S2) for $B \parallel y$ using $g = 65$.

To extract $\alpha$ from our measurements, we fit the model given by equation (S1) and (S2) to the measured gap closing both along the wire and along $B_{\mathrm{SO}}$ simultaneously. We prevent overfitting by independently constraining the free parameters. First, $g$ is determined by the gap closing along $B_{\mathrm{SO}}$, which only depends on the Zeeman effect. Then, $\mu$ follows from the critical field $B_C$ along $x$, where $\frac{1}{2}g\mu_B B_C = \sqrt{\Delta(0)^2 + \mu^2}$ [14, 15] (note that $B_C$ does not depend on $\alpha$). The SOI strength $\alpha$ is now the only free parameter left to fit the curvature of the gap closing along $x$. This procedure is applied to four devices [see Fig. 1(f), Fig. S4(b),(c), and Fig. S7], resulting in a SOI strength of 0.15 – 0.35 eVÅ, corresponding to a spin-orbit energy $E_{\mathrm{SO}} = m^*\alpha^2/2\hbar^2$ of 20 – 120 $\mu$eV. The remaining parameters used for the fit of device A shown in Fig. 1(e) are $g = 90$, $\mu = 1.4$ meV. The values of $g$ and $\mu$ found for the remaining devices are given in Fig. S4. Table I shows the range of values of the fitting parameters for which good fits can be obtained. Since $\alpha$ depends on the electric field in the wire, we expect the observed variation in the SOI strength of devices to be caused by differences in the applied gate voltages and wire diameter.

TABLE S1. Results of gap closing fitting procedure

| | Device A | Device B | Device C | Device D |
|---|---|---|---|---|
| $g$ | 90 ± 10 | 60 ± 20 | 85 ± 5 | 160 ± 20 |
| $\mu$ (meV) | 1.5 ± 0.4 | 1.8 ± 0.8 | 2.75 ± 0.25 | 2.8 ± 0.6 |
| $\alpha$ (eVÅ) | 0.15 ± 0.05 | 0.3 ± 0.1 | 0.35 ± 0.05 | 0.35 ± 0.05 |

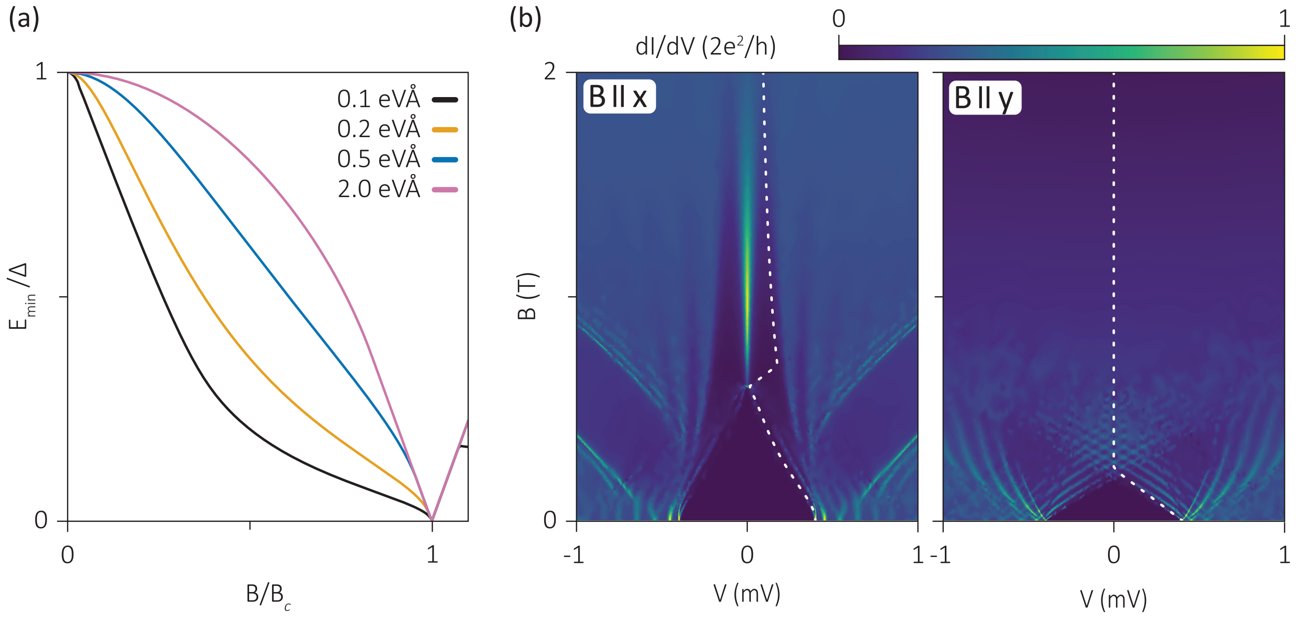


FIG. S2. Extracting SOI strength from gap closing curvature. (a) Lowest energy state $E_{\min}$ determining the gap in the one-dimensional model given by equation S1 as a function of magnetic field, $B$, in units of the critical field $B_c = \sqrt{\Delta^2 + \mu^2}$ for various spin-orbit strengths $\alpha$. The curvature of the gap closing is strongly affected by $\alpha$. Stronger SOI counteracts the Zeeman effect up to larger $B/B_c$, leading initially to a slow gap closing, followed by a sharp gap closing when approaching the critical field, where the lowest energy state is at $k \approx 0$ for which $B_{\mathrm{SO}}(k)$ vanishes. The remaining parameters are: $\Delta(0) = 1$ meV, $\mu = 2$ meV. (b) Comparison of the numerical simulations on the 3D tight binding model, including the orbital effect (color map), with the 1D model given by equations (S1) and (S2) which does not account for the orbital effect (dashed lines). By adjusting the $g$-factor used in the Majorana nanowire model from $g = 50$ to 65 to match the gap closing for $B \parallel B_{\mathrm{SO}}$, keeping all other parameters the same in both models, we find good agreement for the gap closing for $B \parallel x$. We use this same approach to take the orbital effect into account in an effective manner in fits of the experimentally observed gap closing. The remaining parameters used in the simulations shown here are $\Delta(0) = 0.45$ meV, $\mu = 0.95$ meV, $\alpha = 0.2$ eVÅ, $\Delta V_G =$ -10 meV.

**Estimation of SOI strength based on level repulsion**

SOI induces coupling between states of different momentum and spin in finite length Majorana nanowires, which leads to level repulsion when energy levels are nearly degenerate [18]. Recently this level repulsion between longitudinal states within the same subband was used to estimate a SOI strength in epitaxial Al-InSb nanowires [19]. Here, we follow the same procedure to estimate the SOI strength in a seperate device with a NbTiN superconductor that exhibits such level repulsion. We consider a low energy model of two levels dispersing in the magnetic field due to the Zeeman effect, coupled to each other by SOI with the matrix element $\delta_{\mathrm{SO}}$:

$$H = \begin{bmatrix} E_0 + \frac{1}{2} g_0 \mu_B B & \delta_{\mathrm{SO}} \\ \delta_{\mathrm{SO}} & E_1 - \frac{1}{2} g_1 \mu_B B \end{bmatrix} \tag{S3}$$

We fit the eigenenergies of $H$ to our experimental data [Fig. S3a] to extract $\delta_{\mathrm{SO}}$. The precise value of the coupling parameter $\delta_{\mathrm{SO}}$ depends not only on $\alpha$, but also on the details of the confinement and on the coupling strength to the superconductor [19]. A rough estimate, with reasonable agreement to numerical simulations, was proposed to be: $2\delta_{\mathrm{SO}} = \alpha\pi/L$, where $L$ is the length of the wire. The extracted $\delta_{\mathrm{SO}}$ is shown in Fig. S3(b) for various values of the super gate voltage $V_{\mathrm{SG}}$. As $V_{\mathrm{SG}}$ becomes more negative, we see an increase in $\delta_{\mathrm{SO}}$, consistent with an increasing electric field in the nanowire. We can estimate $\alpha \sim 0.4 - 0.55$ eVÅ. Considering the uncertainty in the relation between $\alpha$ and $\delta_{\mathrm{SO}}$ and variation in the electrostatic environment of different devices, this magnitude is in line with our estimation based on the gap closing curvature.

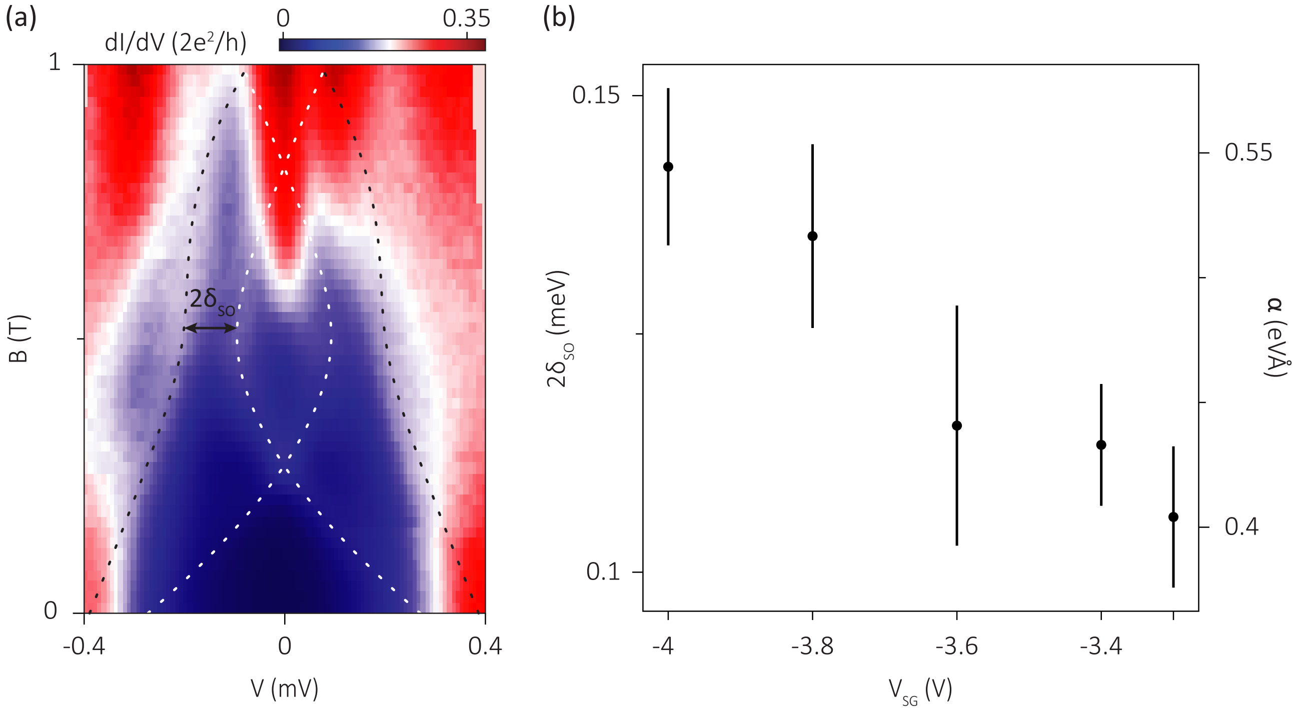


FIG. S3. Extracting the SOI strength from level repulsion. (a) $dI/dV$ as a function of $V$ and $B$ at $V_{\mathrm{SG}}$ = -3.3 V, measured in device E. Two Andreev states come down from the gap edge and exhibit an avoided crossing around $B = 0.5$ T. The dashed lines indicate fits to the solution of equation (S3). The extracted coupling $\delta_{\mathrm{SO}}$ between the Andreev levels is indicated by the arrow. (b) $2\delta_{\mathrm{SO}}$ as a function of $V_{\mathrm{SG}}$. The right axis shows the estimation of the SOI strength using $\alpha = 2\delta_{\mathrm{SO}}L/\pi$ for the 1.2 $\mu$m long superconducting region. The errorbars show the standard deviation in $\delta_{\mathrm{SO}}$ obtained from the fits.

## SUPPLEMENTAL EXPERIMENTAL DATA

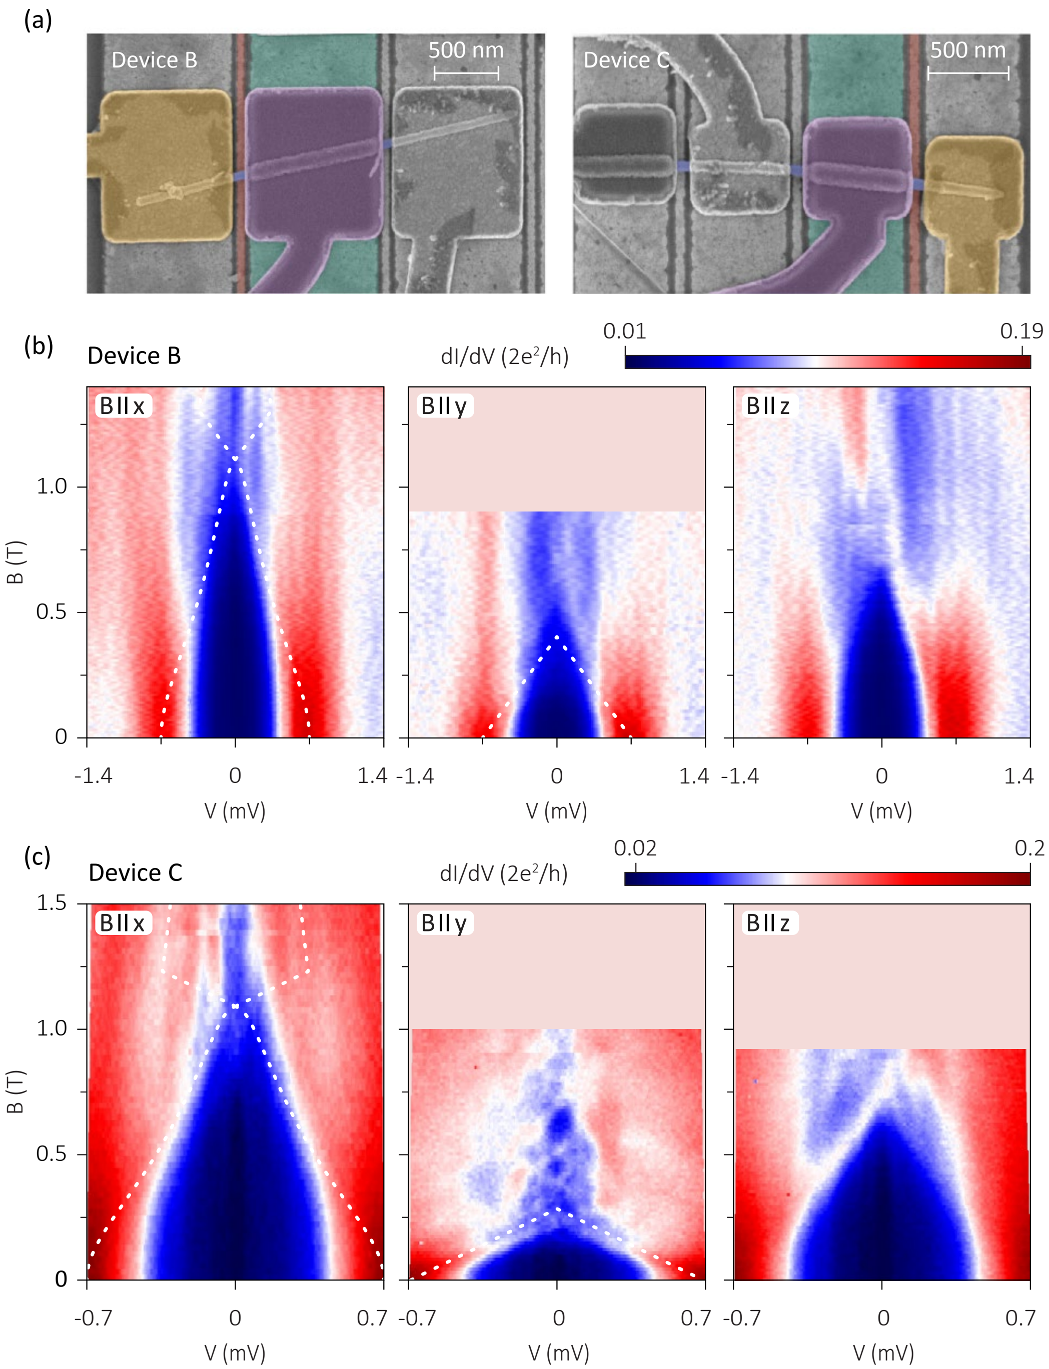


FIG. S4. Anisotropic gap closing in additional devices. (a) False colored scanning electron micrographs of additional devices B (used in Fig. 3) and C, showing anisotropy similar to the device in Fig. 1(e). (b,c) Differential conductance, $dI/dV$, as a function of the magnetic field, $B$, along the $x$, $y$, and $z$-axes (from left to right). The gap closes at much lower fields along the $y$-axis than the $x$ and $z$-axes in all devices fully covered with the superconductor. The white dashed lines indicate fits to the gap closing from which we extract a spin-orbit strength $\alpha$ of 0.3 ± 0.1 eVÅ [for (b)] and 0.35 ± 0.05 eVÅ [for (c)], with $g$ = 60, 85 and $\mu$ = 1.8, 2.7 meV as the remaining fit parameters for (b), (c) respectively. We note that we do not observe clear reopening of the gap in all devices, which theoretical studies have attributed to the negligible contribution to the tunneling conductance of the states associated with the gap reopening due to their spatial wave function extension into the middle of the wire leading to minimal weight near the tunnel barrier [20–23]. The super gate was set to $V_{SG}$ = -1.5 V, -2.6 V in (b), (c) respectively.

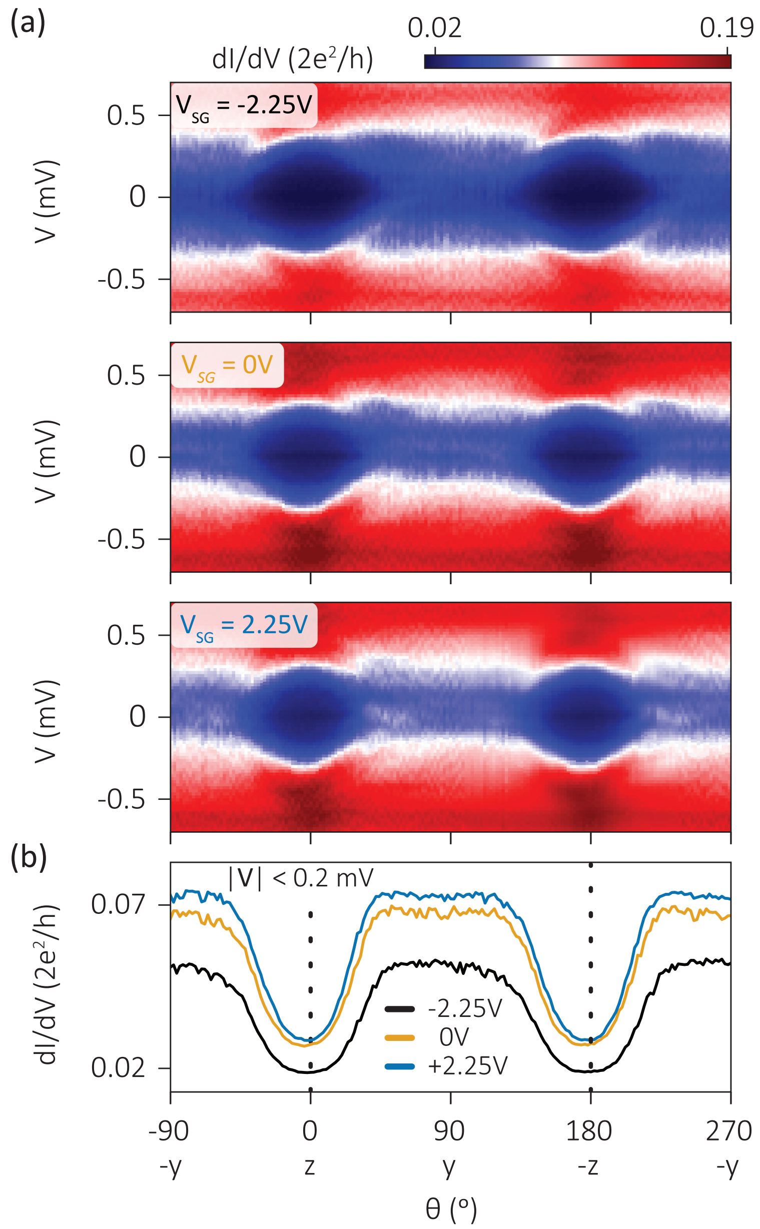


FIG. S5. Gap dependence on magnetic field orientation in $zy$-plane in device A. (a) Differential conductance, $dI/dV$, as a function of bias voltage, $V$, upon rotation of the magnetic field at 0.25 T over angles $\Theta$ between $z$ and $y$ with different voltages on the super gate $V_{\mathrm{SG}}$ in the three panels. This is the same device as presented in Fig 1. (b) Horizontal line cuts of (a) averaged over a bias range $|V| < 0.2$ mV, showing that the hardest gap is at $\Theta = 0$, and increased $V_{\mathrm{SG}}$ suppresses the gap when $B$ is along $y$, the same behaviors observed in device B [Fig. 3].

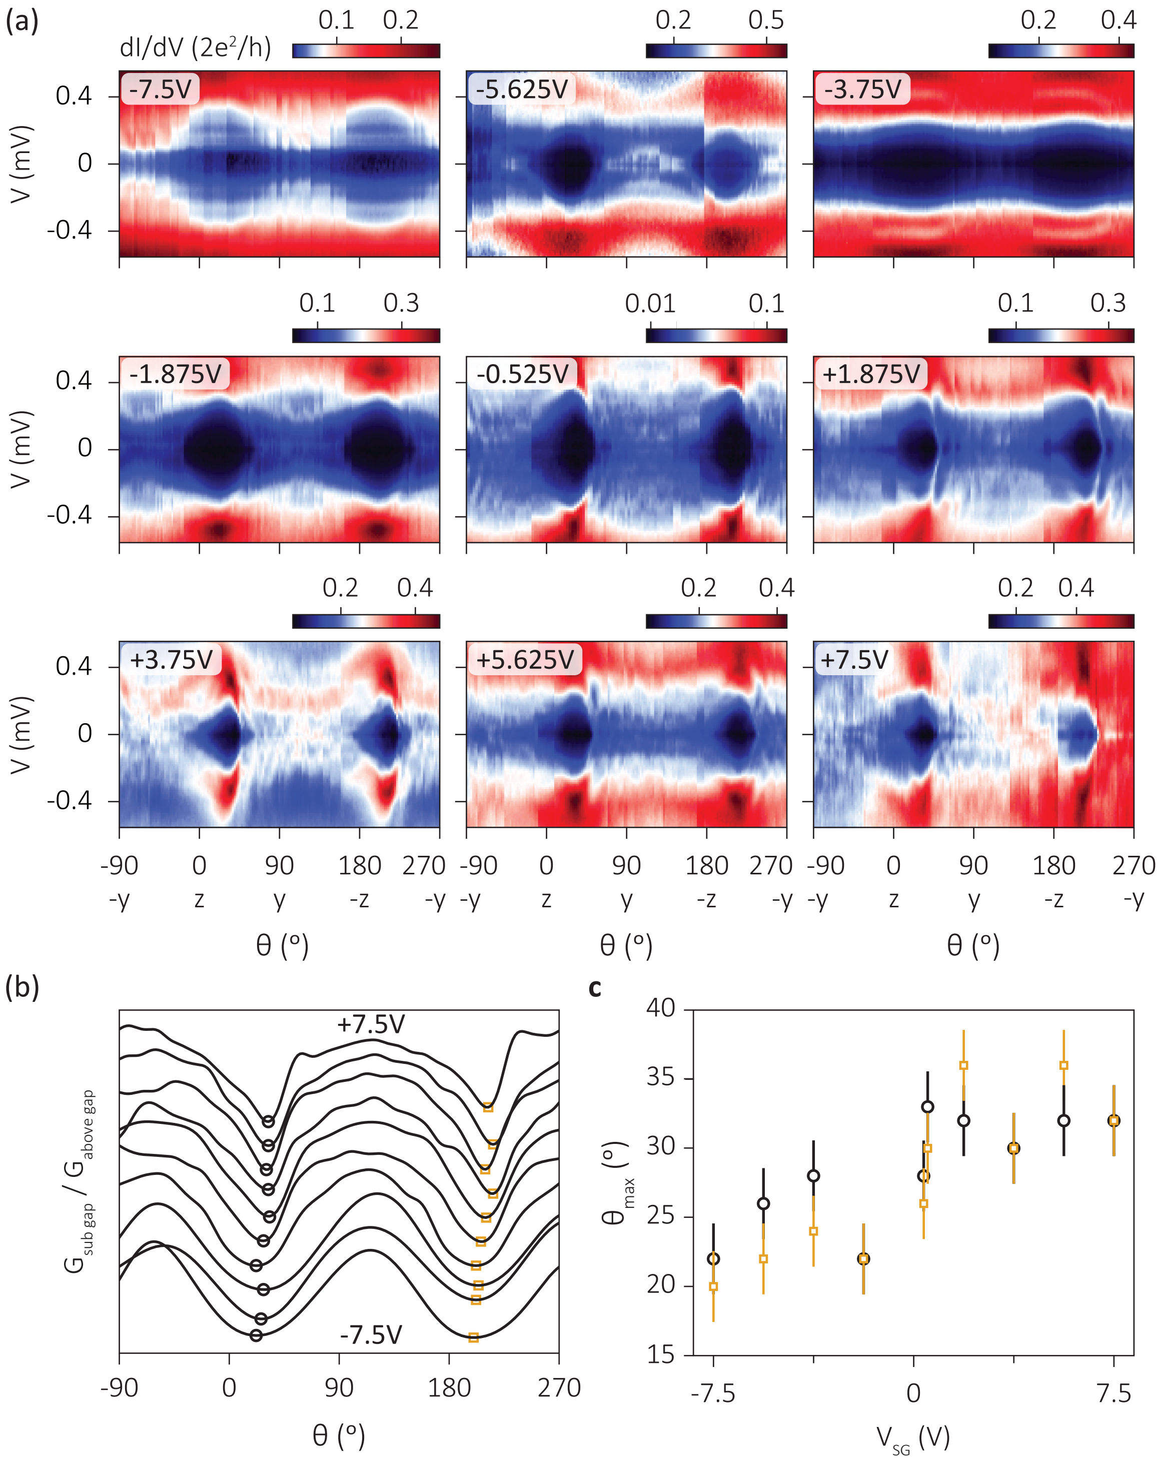


FIG. S6. Dependence of spin-orbit direction on super gate voltage in device D, which is partially covered by NbTiN. (a) Differential conductance, $dI/dV$, as a function of bias voltage, $V$, and angle $\Theta$ between $z$ and $y$ at various values of $V_{\mathrm{SG}}$ as indicated in the insets. The data is measured at slightly different field magnitudes between 0.1 and 0.2 T for the different $V_{\mathrm{SG}}$ to optimize the anisotropy between $y$ and $z$. The discontinuities in $dI/dV$ that are visible for some of the scans are likely caused by charge fluctuations in the dielectric environment. (b) The ratio between the sub gap conductance (averaged over $|V| < 0.2$ V) and the above gap conductance (averaged over $|V| > 0.4$ V) with $V_{\mathrm{SG}}$ increasing from bottom to top and offset for clarity. The minima of the curves signify the angle at which the gap is hardest, $\Theta_{\mathrm{max}}$, which shifts to higher angles at increasing $V_{\mathrm{SG}}$. A lowpass filter is applied along the $\Theta$ direction to suppress the effect of the charge instabilities (this procedure does not affect the minima for the measurements without charge instabilities, such as in Fig. 4). (c) $\Theta_{\mathrm{max}}$ as determined from the first (black) and second (yellow) minimum of the curves in (b) as a function of $V_{\mathrm{SG}}$. The second minima (yellow) signify $\Theta_{\mathrm{max}}$ at negative $B$ and are subtracted by 180° accordingly.

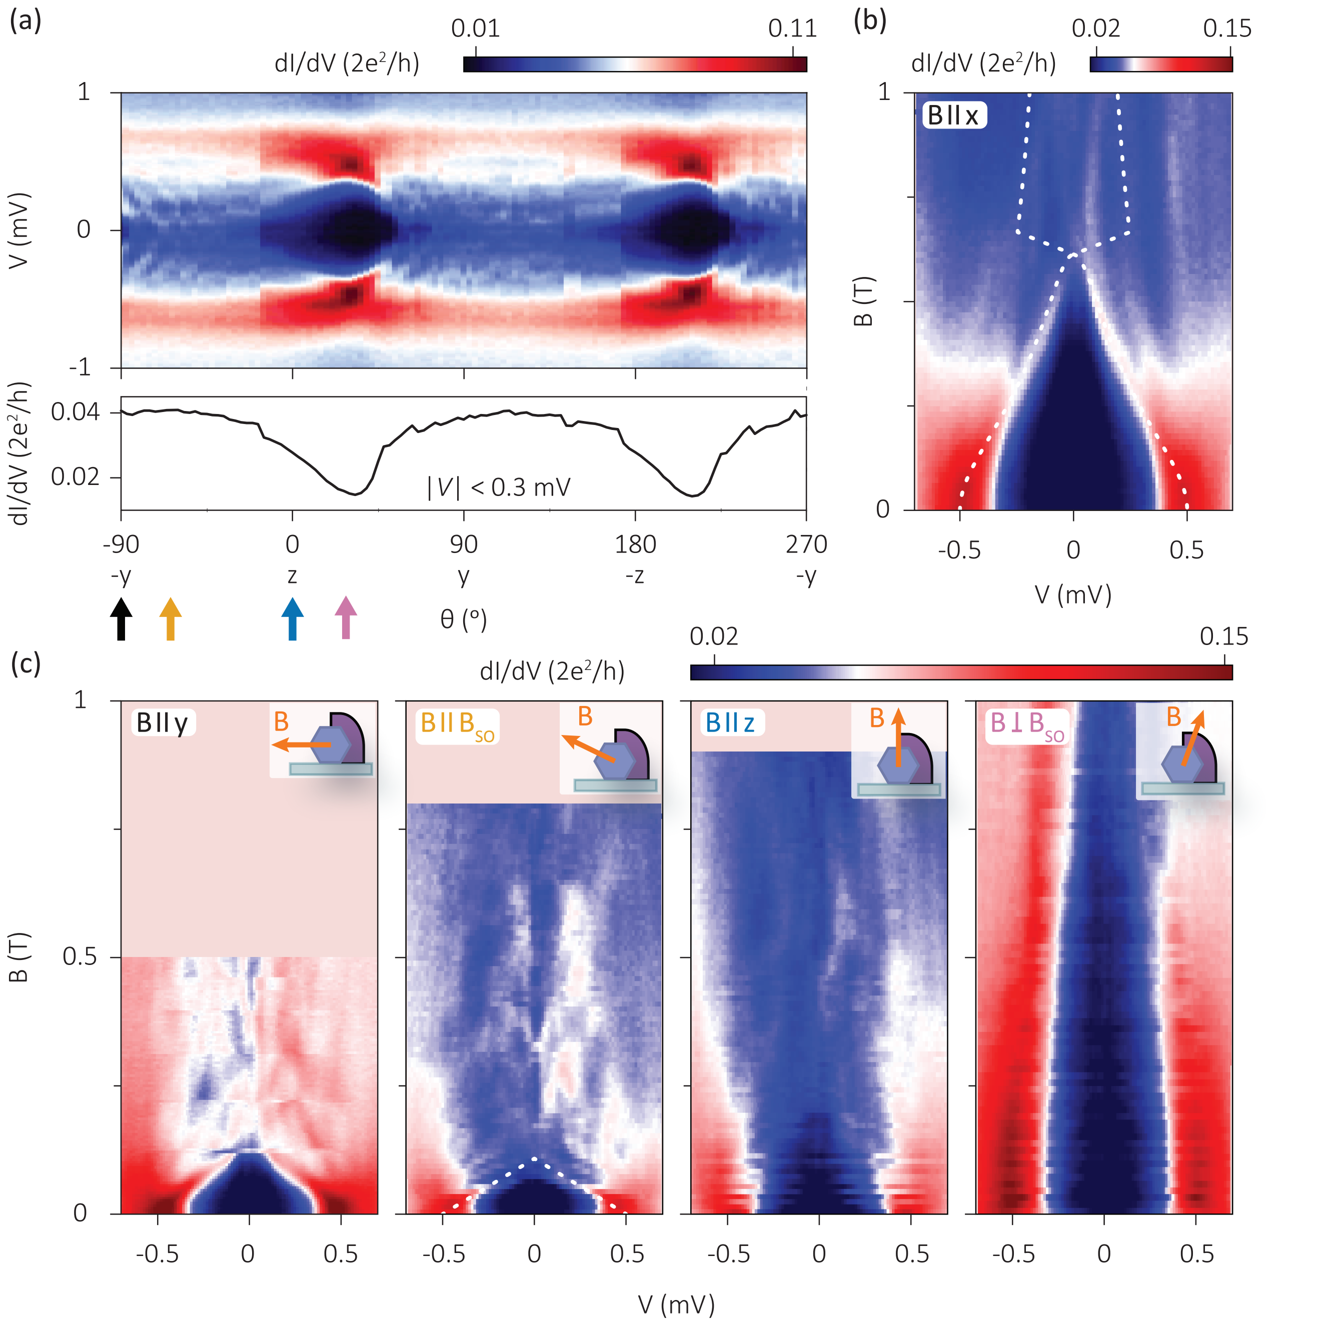


FIG. S7. Gap dependence on magnetic field orientation in device E, which is partially covered by NbTiN. (a) Differential conductance, $dI/dV$, as a function of the angle $\Theta$ between the $z$ and $y$-axes at $V_{\mathrm{SG}} = 0.525$ V and $B = 0.1$ T, with a horizontal line cut averaged over a bias range $|V| < 0.3$ mV in the lower panel. (b) $dI/dV$ as a function of the magnetic field $B$ along the nanowire axis, with the white dashed lines showing the fit to the gap closing, resulting in a spin-orbit strength $\alpha$ of $0.35 \pm 0.05$ eVÅ (the other fit parameters are $g = 160$, see $B \parallel B_{\mathrm{SO}}$ in (c), and $\mu = 2.8$ meV). (c) $dI/dV$ as a function of $B$ along $y$, $B_{\mathrm{SO}}$, $z$ and perpendicular to $B_{\mathrm{SO}}$ from left to right, with the colors in the headers corresponding to the colored arrows in (a). The illustrations in the insets indicate the direction of the magnetic field. Note that due to the changed orientation of $B_{\mathrm{SO}}$, $B$-sweeps along directions rotated by $\sim 25^{\circ}$ from the $y$-axis (second panel, $B \parallel B_{\mathrm{SO}}$) and the $z$-axis (right panel, $B \perp B_{\mathrm{SO}}$) now exhibit strong anisotropy, instead of the $y$ and $z$-axes which show strong anisotropy in devices symmetrically covered by NbTiN.

[1] D. Car, J. Wang, M. A. Verheijen, E. P. A. M. Bakkers, and S. R. Plissard, Rationally designed single-crystalline nanowire networks, Adv. Mater. **26**, 4875 (2014).
[2] K. Flöhr, M. Liebmann, K. Sladek, H. Y. Günel, R. Frielinghaus, F. Haas, C. Meyer, H. Hardtdegen, T. Schäpers, D. Grützmacher, and M. Morgenstern, Manipulating InAs nanowires with submicrometer precision, Rev. Sci. Instrum. **82**, 113705 (2011).
[3] D. B. Suyatin, C. Thelander, M. T. Björk, I. Maximov, and L. Samuelson, Sulfur passivation for ohmic contact formation to InAs nanowires, Nanotechnology **18**, 105307 (2007).
[4] O. Gül, H. Zhang, F. K. de Vries, J. van Veen, K. Zuo, V. Mourik, S. Conesa-Boj, M. P. Nowak, D. J. van Woerkom, M. Quintero-Pérez, M. C. Cassidy, A. Geresdi, S. Koelling, D. Car, S. R. Plissard, E. P. A. M. Bakkers, and L. P. Kouwenhoven, Hard superconducting gap in InSb nanowires, Nano Lett. **17**, 2690 (2017).
[5] H. Zhang, O. Gül, S. Conesa-Boj, M. P. Nowak, M. Wimmer, K. Zuo, V. Mourik, F. K. de Vries, J. van Veen, M. W. A. De Moor, J. D. S. Bommer, D. J. van Woerkom, D. Car, S. R. Plissard, E. P. A. M. Bakkers, M. Quintero-Pérez, M. C. Cassidy, S. Koelling, S. Goswami, K. Watanabe, T. Taniguchi, and L. P. Kouwenhoven, Ballistic superconductivity in semiconductor nanowires, Nat. Commun. **8**, 16025 (2017).
[6] C.-X. Liu, J. D. Sau, and S. Das Sarma, Role of dissipation in realistic Majorana nanowires, Phys. Rev. B **95**, 054502 (2017).
[7] J. Danon, E. B. Hansen, and K. Flensberg, Conductance spectroscopy on Majorana wires and the inverse proximity effect, Phys. Rev. B **96**, 125420 (2017).
[8] B. Nijholt and A. R. Akhmerov, Orbital effect of magnetic field on the Majorana phase diagram, Phys. Rev. B **93**, 235434 (2016).
[9] D. R. Hofstadter, Energy levels and wave functions of Bloch electrons in rational and irrational magnetic fields, Phys. Rev. B **14**, 2239 (1976).
[10] W. D. Gropp, H. G. Kaper, G. K. Leaf, D. M. Levine, M. Palumbo, and V. M. Vinokur, Numerical simulation of vortex dynamics in type-II superconductors, J. Comput. Phys. **123**, 254 (1996).
[11] Q. Du and X. Wu, Numerical solution of the three-dimensional Ginzburg–Landau models using artificial boundary, SIAM J. Numer. Anal. **36**, 1482 (1999).
[12] B. van Heck, J. I. Väyrynen, and L. I. Glazman, Zeeman and spin-orbit effects in the Andreev spectra of nanowire junctions, Phys. Rev. B **96**, 075404 (2017).
[13] H. Pan, J. D. Sau, T. D. Stanescu, and S. Das Sarma, Curvature of gap closing features and the extraction of Majorana nanowire parameters, Phys. Rev. B **99**, 054507 (2019).
[14] R. M. Lutchyn, J. D. Sau, and S. Das Sarma, Majorana fermions and a topological phase transition in semiconductor-superconductor heterostructures, Phys. Rev. Lett. **105**, 077001 (2010).
[15] Y. Oreg, G. Refael, and F. von Oppen, Helical liquids and Majorana bound states in quantum wires, Phys. Rev. Lett. **105**, 177002 (2010).
[16] J. Osca, D. Ruiz, and L. Serra, Effects of tilting the magnetic field in one-dimensional Majorana nanowires, Phys. Rev. B **89**, 245405 (2014).
[17] S. Rex and A. Sudbø, Tilting of the magnetic field in Majorana nanowires: Critical angle and zero-energy differential conductance, Phys. Rev. B **90**, 115429 (2014).
[18] T. D. Stanescu, R. M. Lutchyn, and S. Das Sarma, Dimensional crossover in spin-orbit-coupled semiconductor nanowires with induced superconducting pairing, Physical Rev. B **87**, 094518 (2013).
[19] M. W. A. de Moor, J. D. S. Bommer, D. Xu, G. W. Winkler, A. E. Antipov, A. Bargerbos, G. Wang, N. van Loo, R. L. M. O. het Veld, S. Gazibegovic, D. Car, J. A. Logan, M. Pendharkar, J. S. Lee, E. P. A. M. Bakkers, C. J. Palmstrøm, R. M. Lutchyn, L. P. Kouwenhoven, and H. Zhang, Electric field tunable superconductor-semiconductor coupling in majorana nanowires, New J. of Phys. **20**, 103049 (2018).
[20] E. Prada, P. San-Jose, and R. Aguado, Transport spectroscopy of $NS$ nanowire junctions with Majorana fermions, Phys. Rev. B **86**, 180503 (2012).
[21] F. Pientka, G. Kells, A. Romito, P. W. Brouwer, and F. von Oppen, Enhanced zero-bias Majorana peak in the differential tunneling conductance of disordered multisubband quantum-wire/superconductor junctions, Phys. Rev. Lett. **109**, 227006 (2012).
[22] T. D. Stanescu, S. Tewari, J. D. Sau, and S. Das Sarma, To close or not to close: The fate of the superconducting gap across the topological quantum phase transition in Majorana-carrying semiconductor nanowires, Phys. Rev. Lett. **109**, 266402 (2012).
[23] C.-X. Liu, J. D. Sau, T. D. Stanescu, and S. Das Sarma, Conductance smearing and anisotropic suppression of induced superconductivity in a Majorana nanowire, Phys. Rev. B **99**, 024510 (2019).
